# Supplementary material for: Kanamori-Moir\'e-Hubbard model for transition metal dichalcogenide homobilayers
Source: arXiv:2303.02305 source file (2023-03-04)
Supplement: Supplementary file 1 [file Supplementary.pdf]

**SUPPLEMENTARY INFORMATION** for

# Kanamori-Moiré-Hubbard model for transition metal dichalcogenide homobilayers

by N. Kaushal and E. Dagotto

### Wannierization using the projection technique

We used the projection technique that creates Bloch states with smooth gauge and leads to well-localized Wannier functions. Firstly, the trial wavefunctions ($|g_m\rangle$) are projected onto the manifold of the Bloch states ($|\phi_{m\mathbf{k}}\rangle$) calculated using the continuum model:

$$|\chi_{m\mathbf{k}}\rangle = \sum_{l=1}^{N_B} \langle \phi_{l\mathbf{k}}|g_m\rangle |\phi_{l\mathbf{k}}\rangle, \tag{1}$$

where $N_B$ represents the number of composite bands used i.e. four in our case. The overlap matrix $S(\mathbf{k})$ is defined as $S_{mn}(\mathbf{k}) = \langle \chi_{m\mathbf{k}}|\chi_{n\mathbf{k}}\rangle$. Then, the $S^{-1/2}(\mathbf{k})$ matrix is computed by using $S^{-1/2}(\mathbf{k}) = VD^{-1/2}V^{\dagger}$, where $S(\mathbf{k}) = VDV^{\dagger}$. The overlap matrix is used to construct the unitary transformation $U(\mathbf{k})$, as follows:

$$U_{nl}(\mathbf{k}) = \sum_m \langle \phi_{l\mathbf{k}}|g_m\rangle S^{-1/2}_{mn}(\mathbf{k}). \tag{2}$$

Using the above unitary transformation, new Bloch states with smooth gauge can be calculated which can be used to obtain well-localized Wannier functions ($|\Psi_n\rangle$):

$$|\tilde{\phi}_{n\mathbf{k}}\rangle = \sum_l U_{nl}(\mathbf{k})|\phi_{l\mathbf{k}}\rangle \tag{3}$$

$$|\Psi_n\rangle = \frac{1}{\sqrt{\tilde{l}_1\tilde{l}_2}} \sum_{\mathbf{k}} |\tilde{\phi}_{n\mathbf{k}}\rangle \tag{4}$$

where, $\tilde{l}_1$ and $\tilde{l}_2$ are the total number of points in the moiré Brillouin zone in the direction of reciprocal lattice vectosr $\mathbf{g}_1 = \frac{2\pi}{a_m}(\frac{1}{\sqrt{3}}, -1)$ and $\mathbf{g}_2 = \frac{2\pi}{a_m}(\frac{1}{\sqrt{3}}, 1)$, respectively. The typical moiré crystal momentum is given by $\mathbf{k} = \frac{n_1}{\tilde{l}_1}\mathbf{g}_1 + \frac{n_2}{\tilde{l}_2}\mathbf{g}_2$.

We used the hydrogen atom $p$-orbital eigenfunctions as trial wave functions, which resembles the target Wannier functions. We found this technique produces well localized and real Wannier functions.

### Calculating hopping parameters and longer-range hopping terms

The elements of $2 \times 2$ hopping matrices required to construct the tight-binding model are defined as $t^{SS'}_{\mathbf{j}-\mathbf{i}}(\mu,\nu) = \langle \Psi^{\mathbf{j}}_{S\mu}|H|\Psi^{\mathbf{i}}_{S'\nu}\rangle$. Because the Wannier fuctions are not the eigenstates of the Hamiltonian, thus we use Eq. 4 followed by Eq. 3, and use $H|\phi_{n\mathbf{k}}\rangle = \epsilon^{\mathbf{k}}_n|\phi_{n\mathbf{k}}\rangle$ to obtain

$$t^{SS'}_{\mathbf{j}-\mathbf{i}}(\mu,\nu) = \frac{1}{\tilde{l}_1\tilde{l}_2} \sum_{\mathbf{k}n} \epsilon^{\mathbf{k}}_n (U^{\mathbf{k}}(S_\mu, n))^* U^{\mathbf{k}}(S'_\nu, n) e^{i\mathbf{k}\cdot(\mathbf{R_j}-\mathbf{R_i})}. \tag{5}$$

We checked the convergence of the Wannier functions with increasing number of momentum points ($\tilde{l}_1\tilde{l}_2$) in the moiré Brillouin zone, and found that already $\tilde{l}_1\tilde{l}_2$=81 and 144 give the same results.

Using Eq. 5 we calculated the hoppings until the 3rd-nearest neighbour distance. In the main paper we only showed the nearest-neighbour hopping term ($K^1_{\mathbf{i}\sigma}$). Below, we show the 2nd ($K^2_{\mathbf{i}\sigma}$) and 3rd ($K^3_{\mathbf{i}\sigma}$) nearest-neighbour terms.

$$K^2_{\mathbf{i}\sigma} = \sum_{\substack{\nu,\mu\in\{p_x,p_y\} \\ S\in\{A,B\} \\ \mathbf{r}\in\{\mathbf{a_1},-\mathbf{a_2},\mathbf{a_1}-\mathbf{a_2}\}}} t^{SS}_{\mathbf{r}}(\mu,\nu) c^{\dagger}_{\mathbf{i}+\mathbf{r}S_\mu\sigma} c_{\mathbf{i}S_\nu\sigma} + h.c. \tag{6}$$

$$K^3_{\mathbf{i}\sigma} \;=\; \sum_{\substack{\nu,\mu\in\{p_x,p_y\}\\ S\in\{A,B\}}} t^{S\bar{S}}_{\mathbf{a_1}}(\mu,\nu)c^\dagger_{\mathbf{i}+\mathbf{a}_1 S_\mu\sigma}c_{\mathbf{i}\bar{S}_\nu\sigma} \;+\; \sum_{\nu,\mu\in\{p_x,p_y\}} t^{BA}_{\mathbf{a}_1-2\mathbf{a}_2}(\mu,\nu)c^\dagger_{\mathbf{i}+\mathbf{a}_1-2\mathbf{a}_2B_\mu\sigma}c_{\mathbf{i}A_\nu\sigma} \;+\; h.c. \quad (7)$$

We present all the hopping matrices for the twist angles 1.0 and 2.0 in tabular form, showing that just nearest neighbour hopping matrices are sufficient for small twist angles like $\theta = 1.0$, but longer-range hoppings are required for the larger twist angles to correctly capture the band structure.

TABLE I. Hopping parameters for twist angles $\theta = 1.0$ and $\theta = 2.5$ ($0 < \epsilon \le \mathcal{O}(10^{-3})$).

| | $\theta = 1.0$ | $\theta = 2.5$ |
|---|---|---|
| $t^{BA}_{\mathbf{0}}$ | $\begin{pmatrix}-0.031 & -0.106\\ -0.106 & -0.154\end{pmatrix}$ | $\begin{pmatrix}-0.869 & -5.912\\ -5.912 & -7.695\end{pmatrix}$ |
| $t^{BA}_{-\mathbf{a_2}}$ | $\begin{pmatrix}-0.216 & 0\\ 0 & 0.030\end{pmatrix}$ | $\begin{pmatrix}-11.107 & 0\\ 0 & 2.545\end{pmatrix}$ |
| $t^{BA}_{\mathbf{a_1}-\mathbf{a_2}}$ | $\begin{pmatrix}-0.031 & 0.106\\ 0.106 & -0.154\end{pmatrix}$ | $\begin{pmatrix}-0.869 & 5.912\\ 5.912 & -7.695\end{pmatrix}$ |
| $t^{AA}_{\mathbf{a_1}}$ | $\begin{pmatrix}\epsilon & \epsilon\\ \epsilon & \epsilon\end{pmatrix}$ | $\begin{pmatrix}0.611 & 0.291\\ -0.289 & 0.613\end{pmatrix}$ |
| $t^{AA}_{-\mathbf{a_2}}$ | $\begin{pmatrix}\epsilon & \epsilon\\ \epsilon & \epsilon\end{pmatrix}$ | $\begin{pmatrix}0.611 & 0.289\\ -0.291 & 0.613\end{pmatrix}$ |
| $t^{AA}_{\mathbf{a_1}-\mathbf{a_2}}$ | $\begin{pmatrix}\epsilon & \epsilon\\ \epsilon & \epsilon\end{pmatrix}$ | $\begin{pmatrix}0.614 & -0.290\\ 0.290 & 0.611\end{pmatrix}$ |
| $t^{BB}_{\mathbf{a_1}}$ | $\begin{pmatrix}\epsilon & \epsilon\\ \epsilon & \epsilon\end{pmatrix}$ | $\begin{pmatrix}0.612 & -0.289\\ 0.292 & 0.613\end{pmatrix}$ |
| $t^{BB}_{-\mathbf{a_2}}$ | $\begin{pmatrix}\epsilon & \epsilon\\ \epsilon & \epsilon\end{pmatrix}$ | $\begin{pmatrix}0.612 & -0.292\\ 0.289 & 0.613\end{pmatrix}$ |
| $t^{BB}_{\mathbf{a_1}-\mathbf{a_2}}$ | $\begin{pmatrix}\epsilon & \epsilon\\ \epsilon & \epsilon\end{pmatrix}$ | $\begin{pmatrix}0.613 & 0.290\\ -0.290 & 0.611\end{pmatrix}$ |
| $t^{AB}_{\mathbf{a_1}}$ | $\begin{pmatrix}\epsilon & \epsilon\\ \epsilon & \epsilon\end{pmatrix}$ | $\begin{pmatrix}0.484 & 0.424\\ 0.424 & \epsilon\end{pmatrix}$ |
| $t^{BA}_{\mathbf{a_1}}$ | $\begin{pmatrix}\epsilon & 0\\ 0 & \epsilon\end{pmatrix}$ | $\begin{pmatrix}-0.251 & 0\\ 0 & 0.729\end{pmatrix}$ |
| $t^{BA}_{\mathbf{a_1}-2\mathbf{a_2}}$ | $\begin{pmatrix}\epsilon & \epsilon\\ \epsilon & \epsilon\end{pmatrix}$ | $\begin{pmatrix}0.484 & -0.424\\ -0.424 & \epsilon\end{pmatrix}$ |

### Calculation of the interaction parameters

The generic four-fermionic interaction parameter can be written as follows,

$$V^{\alpha\beta\gamma\delta}_{\mathbf{ijkl}} = \langle R^\alpha_{\mathbf{i}} R^\beta_{\mathbf{j}}|V|R^\gamma_{\mathbf{k}} R^\delta_{\mathbf{l}}\rangle = \int d^2\mathbf{r}d^2\mathbf{r}'\Psi^{\mathbf{i}*}_\alpha(\mathbf{r})\Psi^{\mathbf{j}*}_\beta(\mathbf{r}')V(\mathbf{r}-\mathbf{r}')\Psi^{\mathbf{k}}_\gamma(\mathbf{r})\Psi^{\mathbf{l}}_\delta(\mathbf{r}'), \quad (8)$$

where $V(\mathbf{r}-\mathbf{r}') = \frac{e^2}{\epsilon|\mathbf{r}-\mathbf{r}'|}$. Direct numerical integration of the above equation is costly as there are 4 variables for integration ($r_{x(y)}$ and ${r'}_{x(y)}$) and there is a singularity for $\mathbf{r} = \mathbf{r}'$. Thus, we transform the above equation into momentum space and obtain

$$V^{\alpha\beta\gamma\delta}_{\mathbf{ijkl}} = \frac{1}{(2\pi)^2}\int d^2\mathbf{q}V(\mathbf{q})e^{i\mathbf{q}\cdot(\mathbf{R_j}-\mathbf{R_k})}M^*_{\gamma\alpha}(\mathbf{q},\mathbf{R_k}-\mathbf{R_i})M_{\delta\beta}(\mathbf{q},\mathbf{R_j}-\mathbf{R_l}), \quad (9)$$

where $M_{\gamma,\alpha}(\mathbf{q},\mathbf{R}) = \int d^2\mathbf{r}\Psi^*_\gamma(\mathbf{r})\Psi_\alpha(\mathbf{r}+\mathbf{R})e^{i\mathbf{q}\cdot\mathbf{r}}$ and $V(\mathbf{q}) = \frac{2\pi e^2}{\epsilon q}$. Furthermore, we perform the integration in spherical coordinates to get rid of the divergence at $\mathbf{q} = 0$ by substituting $d^2\mathbf{q}V(\mathbf{q})$ to $2\pi dqd\theta e^2/\epsilon$. Using the above, we calculated all the interaction parameters up to the nearestneighbour in the honeycomb lattice.

## Nearest-neighbour interaction terms of KMH model

In the main text, we only showed the intra-unit cell Coulomb interaction terms, which also includes interactions with one of the three nearest-neighbour sites of the honeycomb lattice. In this section, we discuss the interaction terms with the other 2 nearest-neighbours. Below, we show an interaction term between the sites belonging to sublattice $A$ of unit cell $\mathbf{i}$ and sublattice $B$ of unit cell $\mathbf{j}$:

$$
\begin{aligned}
H^{AB}_{\mathbf{ij}} = & \sum_{\substack{\alpha\in 01\\ \beta\in 23}} \Big(U^{\mathbf{ij}}_{\alpha\beta} - \frac{J^{\mathbf{ij}}_{\alpha\beta}}{2}\Big) n_{\mathbf{i}\alpha} n_{\mathbf{j}\beta} - 2\sum_{\substack{\alpha\in 01\\ \beta\in 23}} J^{\mathbf{ij}}_{\alpha\beta} \mathbf{S}_{\mathbf{i}\alpha}\cdot\mathbf{S}_{\mathbf{j}\beta} + \sum_{\substack{\alpha\in 01\\ \beta\in 23}} J^{\mathbf{ij}}_{\alpha\beta}(P^{\dagger}_{\mathbf{i}\alpha} P_{\mathbf{j}\beta} + h.c.) + \sum_{\substack{\sigma,\mathbf{l}\neq\mathbf{n}\\ \mathbf{l},\mathbf{n}\in\{\mathbf{i},\mathbf{j}\}\\ \alpha_{\mathbf{i}}\in 01,\alpha_{\mathbf{j}}\in 23}} \tilde{A}^{\mathbf{ln}}_{\alpha_{\mathbf{l}}\alpha_{\mathbf{n}}} (c^{\dagger}_{\mathbf{l}\alpha_{\mathbf{l}}\sigma} c_{\mathbf{n}\alpha_{\mathbf{n}}\sigma} n_{\mathbf{n}\alpha_{\mathbf{n}}\bar{\sigma}} + h.c.) \\
& + 1/2 \sum_{\substack{\sigma,\sigma',\mathbf{l}\neq\mathbf{n}\neq\mathbf{m},\\ \mathbf{l},\mathbf{n},\mathbf{m}\in\{\mathbf{i},\mathbf{j}\},\\ \alpha_{\mathbf{i}}\in 01,\alpha_{\mathbf{j}}\in 23}} (A^{\mathbf{nlm}}_{\alpha_{\mathbf{n}}\alpha_{\mathbf{l}}\alpha_{\mathbf{m}}} - \delta_{\sigma\sigma'} \tilde{J}^{\mathbf{nlm}}_{\alpha_{\mathbf{n}}\alpha_{\mathbf{l}}\alpha_{\mathbf{m}}})(c^{\dagger}_{\mathbf{l}\alpha_{\mathbf{l}}\sigma} c_{\mathbf{m}\alpha_{\mathbf{m}}\sigma} n_{\mathbf{n}\alpha_{\mathbf{n}},\sigma'} + h.c.) + 1/2 \sum_{\substack{\sigma,\mathbf{l}\neq\mathbf{n}\neq\mathbf{m},\\ \mathbf{l},\mathbf{n},\mathbf{m}\in\{\mathbf{i},\mathbf{j}\},\\ \alpha_{\mathbf{i}}\in 01,\alpha_{\mathbf{j}}\in 23}} \tilde{J}^{\mathbf{lmn}}_{\alpha_{\mathbf{l}}\alpha_{\mathbf{m}}\alpha_{\mathbf{n}}} s(P^{\dagger}_{\mathbf{l}\alpha_{\mathbf{l}}} c_{\mathbf{m}\alpha_{\mathbf{m}}\bar{\sigma}} c_{\mathbf{n}\alpha_{\mathbf{n}}\sigma} + h.c.) \\
& - \sum_{\substack{\mathbf{l}\neq\mathbf{n}\neq\mathbf{m},\\ \mathbf{l},\mathbf{n},\mathbf{m}\in\{\mathbf{i},\mathbf{j}\},\\ \alpha_{\mathbf{i}}\in 01,\alpha_{\mathbf{j}}\in 23}} \tilde{J}^{\mathbf{lmn}}_{\alpha_{\mathbf{l}}\alpha_{\mathbf{m}}\alpha_{\mathbf{n}}} (S^{+}_{\mathbf{l}\alpha_{\mathbf{l}}} c^{\dagger}_{\mathbf{n}\alpha_{\mathbf{n}}\downarrow} c_{\mathbf{m}\alpha_{\mathbf{m}}\uparrow} + h.c.) + \sum_{\substack{\sigma,\sigma',\\ \{\mathbf{l}\alpha_{\mathbf{l}},\mathbf{n}\alpha_{\mathbf{n}},\mathbf{m}\alpha_{\mathbf{m}},\mathbf{p}\alpha_{\mathbf{p}}\}\in\mathbb{S}'}} T^{\mathbf{lnmp}}_{\alpha_{\mathbf{l}}\alpha_{\mathbf{n}}\alpha_{\mathbf{m}}\alpha_{\mathbf{p}}} (c^{\dagger}_{\mathbf{l}\alpha_{\mathbf{l}}\sigma} c_{\mathbf{m}\alpha_{\mathbf{m}}\sigma} (c^{\dagger}_{\mathbf{n}\alpha_{\mathbf{n}}\sigma'} c_{\mathbf{p}\alpha_{\mathbf{p}}\sigma'} + c^{\dagger}_{\mathbf{p}\alpha_{\mathbf{p}}\sigma'} c_{\mathbf{n}\alpha_{\mathbf{n}}\sigma'}) + h.c.)
\end{aligned}
\tag{10}
$$

The above expression can depict the rest of the 2 nearest-neighbour interactions when $\mathbf{j} = \mathbf{i} - \mathbf{a}_2$ and $\mathbf{j} = \mathbf{i} + \mathbf{a}_1 - \mathbf{a}_2$. The above terms are exactly similar to the terms present in the main paper, except here the local interactions are absent to avoid the double counting. The $\mathbf{l} \neq \mathbf{n} \neq \mathbf{m}$ is short hand notation for $\mathbf{l} \neq \mathbf{n}$, $\mathbf{n} \neq \mathbf{m}$, and $\mathbf{m} \neq \mathbf{l}$. The set is $\mathbb{S}' = \{(\mathbf{i}0, \mathbf{i}1, \mathbf{j}2, \mathbf{j}3), (\mathbf{i}0, \mathbf{i}1, \mathbf{j}3, \mathbf{j}2), (\mathbf{i}0, \mathbf{j}2, \mathbf{i}1, \mathbf{j}3)\}$

In Fig. 1, we show the evolution of the $\tilde{J}_{\alpha\gamma\beta}$ and $T_{\alpha\beta\gamma\delta}$ parameters, which were not shown in the main paper.

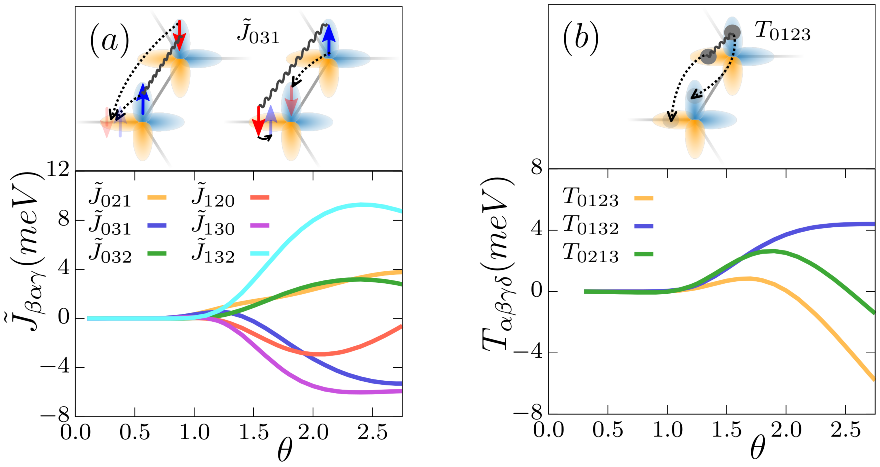


FIG. 1. Panels (a) and (b) show the evolution of the $\tilde{J}_{\alpha\gamma\beta}$ and $T_{\alpha\beta\gamma\delta}$ parameters (present in the term $H_{\mathbf{i}}$) vs. $\theta$, repectively.

### Unrestricted Hartree-Fock details

We performed the Hartree-Fock directly on Eq. 2 of the main paper. Thus, the mean field Hamiltonian can be written as follows:

$$H_{Hartree} = \frac{1}{2}\sum_{\substack{\mathbf{ijkl}\\ \alpha\beta\gamma\delta\\ \sigma\sigma'}} V^{\alpha\beta\gamma\delta}_{\mathbf{ijkl}}(\langle c^{\dagger}_{\mathbf{i}\alpha\sigma}c_{\mathbf{k}\gamma\sigma}\rangle c^{\dagger}_{\mathbf{j}\beta\sigma'}c_{\mathbf{l}\delta\sigma'} + \langle c^{\dagger}_{\mathbf{j}\beta\sigma'}c_{\mathbf{l}\delta\sigma'}\rangle c^{\dagger}_{\mathbf{i}\alpha\sigma}c_{\mathbf{k}\gamma\sigma} - \langle c^{\dagger}_{\mathbf{i}\alpha\sigma}c_{\mathbf{k}\gamma\sigma}\rangle\langle c^{\dagger}_{\mathbf{j}\beta\sigma'}c_{\mathbf{l}\delta\sigma'}\rangle) - \frac{1}{2}\sum_{\substack{\mathbf{ijjl}\\ \alpha\beta\delta\\ \sigma}} V^{\alpha\beta\beta\delta}_{\mathbf{ijjl}} c^{\dagger}_{\mathbf{j}\alpha\sigma}c_{\mathbf{l}\delta\sigma} \tag{11}$$

$$H_{Fock} = -\frac{1}{2}\sum_{\substack{\mathbf{ijkl}\\ \alpha\beta\gamma\delta\\ \sigma\sigma'}} (V^{\alpha\beta\gamma\delta}_{\mathbf{ijkl}} + V^{\alpha\beta\delta\gamma}_{\mathbf{ijlk}})\langle c^{\dagger}_{\mathbf{i}\alpha\sigma}c_{\mathbf{l}\delta\sigma'}\rangle c^{\dagger}_{\mathbf{j}\beta\sigma'}c_{\mathbf{k}\gamma\sigma} - V^{\alpha\beta\gamma\delta}_{\mathbf{ijkl}}\langle c^{\dagger}_{\mathbf{i}\alpha\sigma}c_{\mathbf{l}\delta\sigma'}\rangle\langle c^{\dagger}_{\mathbf{j}\beta\sigma'}c_{\mathbf{k}\gamma\sigma}\rangle + \sum_{\substack{\mathbf{ijk}\\ \alpha\beta\gamma\\ \sigma}} V^{\alpha\beta\gamma\beta}_{\mathbf{ijkj}} c^{\dagger}_{\mathbf{i}\alpha\sigma}c_{\mathbf{k}\gamma\sigma} \tag{12}$$

We started from 10-15 random initial values for the order parameters, and chose the converged solution with the lowest energy as the ground state. A convergence error of $10^{-5}$ was used. We used the Anderson-mixing method for accelerated convergence. We also performed the unrestricted Hartree-Fock calculations using the recently developed hybrid momentum-real space Hartree-Fock technique where the specific translational symmetry sectors can be targetted [1], and we found the same results discussed in the main text.

[1] N. Kaushal, N. M.-Durán, A. H. MacDonald, and E. Dagotto, Comm. Phys. **4**, 289 (2022) .
